# Supplementary material for: Seeding Method for Ice Nucleation under Shear
Source: arXiv:2006.14919 source file (2020-08-06)
Supplement: Supplementary file 1 [file supplementary.pdf]

# Supporting Information: Seeding Method for Ice Nucleation under Shear

Amrita Goswami, Indranil Saha Dalal,* and Jayant K. Singh*

*Department of Chemical Engineering, Indian Institute of Technology Kanpur*

E-mail: indrasd@iitk.ac.in; jayantks@iitk.ac.in

## 1 The Seeding Technique: Calculation of $N^*$

In this work, we have extended the Classical Nucleation Theory (CNT) equations, explicitly accounting for the effects of volume-preserving simple shear flows. In our formalism, the interfacial energy $\nu_0$ and chemical potential difference $|\Delta\mu_0|$ in the absence of shear, along with the shear modulus $G$, viscosity $\eta$, density of the liquid and solid phases and the diffusion coefficient $D_l$ are the input parameters required to solve the modified CNT equations.

The seeding technique[S1,S2] enables the direct determination of the critical nucleus size $N^*$ at a particular temperature. The estimated $N^*$ is then typically used to calculate the interfacial energy $\nu_0$, within the framework of CNT.

Thus, the use of the seeding technique in our methodology is to determine $\nu_0$ at the given thermodynamic conditions. $\nu_0$ is subsequently used as one of the inputs for calculating the free energy barrier height and nucleation rate.

In the seeding method, a seed of a known size is inserted into a supercooled liquid. The size of the inserted seed is monitored at trial temperatures. The temperature at which the cluster grows for roughly half of the trajectories and shrinks in the rest is the temperature at which the cluster size is critical.

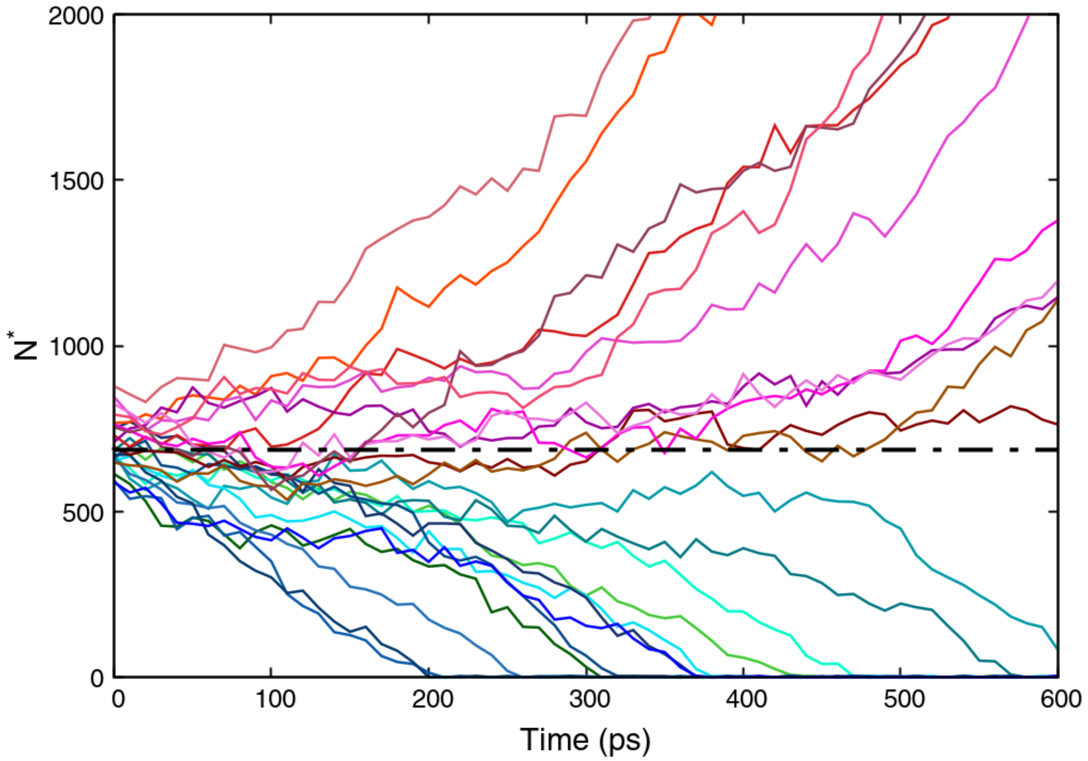


Figure S1: Cluster size time evolution for an initial seed size of 686 particles, at 240 $K$ and 1 $atm$ pressure. The mW water model was used. The black dotted line denotes the initial cluster size.

Figure S1 depicts the time evolution of the number of particles in the largest ice cluster, at 240 $K$ and 1 $atm$. The size of the initial cluster was approximately 686 particles, which is the critical size at this temperature. Out of about 30 independent trajectories, the cluster grows and fills the box in roughly half the runs, while the cluster shrinks and disappears in the rest.

## 2 Input Parameters

Seeding method data, fluid properties and the chemical potential are input parameters used for the modified CNT equations presented in this work. Table S1 lists the input parameters for the mW water model.[S3]

The seeding method results were obtained by observing the growth of inserted clusters

($N^*$) in supercooled liquid configurations. The total size of each system is denoted by $N_T$. The system size is chosen such that it is $\approx 20$ times the number of molecules in the inserted cluster. The interfacial energy $\nu_0$ is thus estimated from the expression for $N^*$, using the CNT framework.

The chemical potential $\Delta\mu_0$ for each temperature has been taken from Espinosa et al.[S4] and.[S5] The viscosities $\eta$ have been obtained from Dehaoui et al.[S6]. The shear modulus $G$ has been taken to be 3.5 $GPa$.[S7] The jump length $\lambda$ used is 3.5 Å. The density of the liquid is $\rho_l$ and the volume occupied by one ice molecule is $v'$.

Table S1: Parameters for the mW water model

| $T$ (K) | $N^*$ | $N_T$ | $\nu_0$ $(mN/m)$ | $\Delta\mu_0$ $(kcal/mol)$ | $\eta$ $(cP)$ | $\rho_l$ $(g/cm^3)$ |
|---|---|---|---|---|---|---|
| 235 | 435 | 19360 | 30.15 | 0.18 | 25.88 | 1.0031 |
| 240 | 688 | 22759 | 30.28 | 0.1553 | 12.68 | 1.0031 |
| 255 | 3501 | 76781 | 30.0 | 0.0895 | 3.967 | 1.0024 |
| 260 | 8277 | 182,585 | 29.85 | 0.0669 | 3.059 | 1.0022 |

## 3 Supplementary Figures and Tables

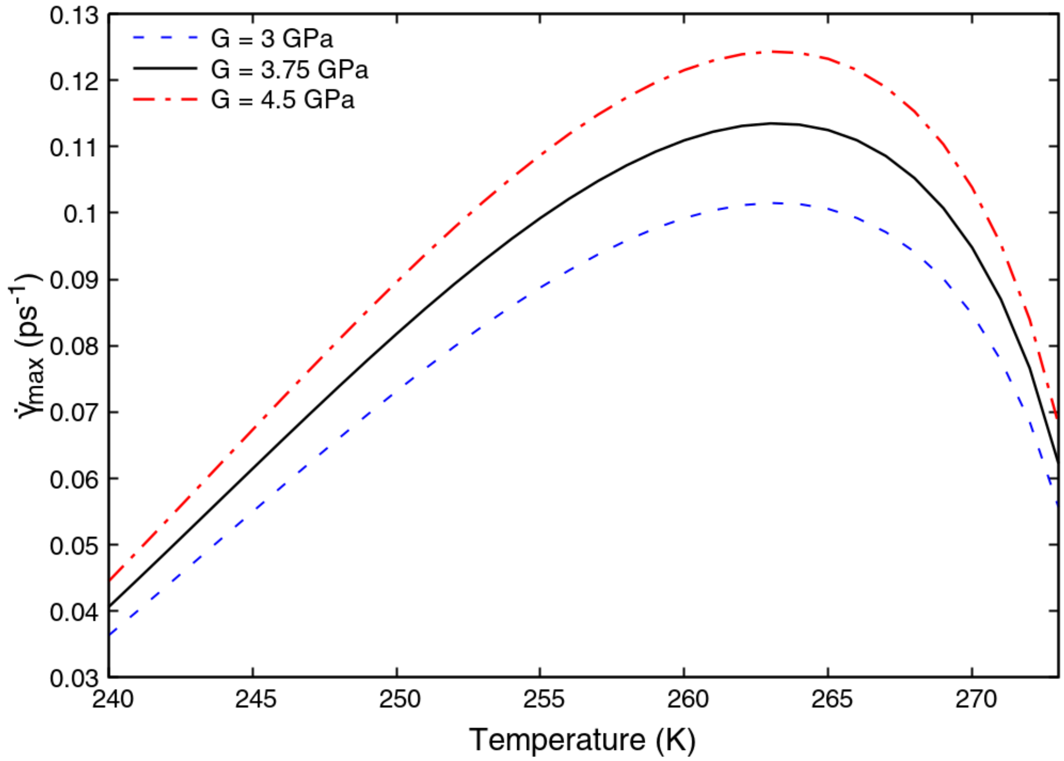


Figure S2: Temperature dependence of $\dot{\gamma}_{max}$ for the mW water model, calculated using approximations for $\eta$ and $|\Delta\mu|$, for different values of $G$. The shear moduli of ice nuclei have been reported to vary within the range of $\approx 3 - 4.5$ $GPa$, exhibiting anisotropy due to structural differences and the crystal plane direction.[S7–S9] $\dot{\gamma}_{max}$ has been plotted for $G = 3$ $GPa$ (dotted blue line), $G = 3.75$ $GPa$ (solid black line) and $G = 4.5$ $GPa$ (dotted red line). $\dot{\gamma}_{max}$ calculated for $G = 3$ $GPa$ and $G = 4.75$ $GPa$ vary by about $\approx 10\%$ from the values determined using $G = 3.75$ $GPa$. In this work, we have used a constant value of $G = 3.1$ $GPa$, corresponding to the shear modulus calculated for an amorphous ice cluster, simulated using the mW model.[S7] We also note that $\dot{\gamma}_{max}$ has a maxima at about 263 $K$ for all three values of $G$.

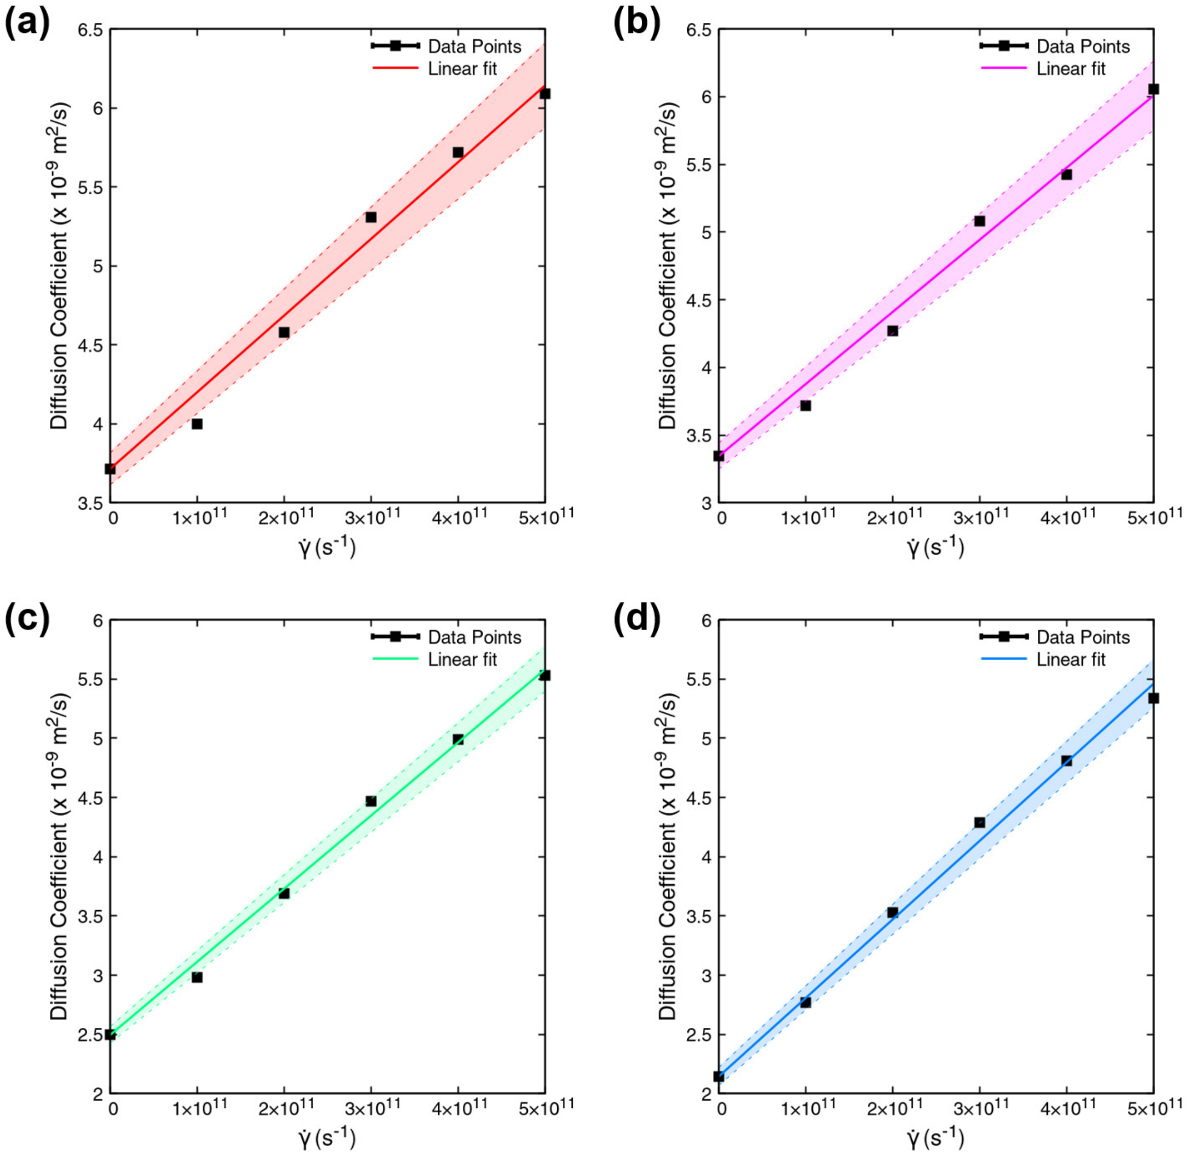


Figure S3: Linear fits of diffusion coefficients at different shear rates at constant temperature, for a) 260 K, (b) 255 K, (c) 240 K and (d) 235 K. In each plot, the filled black squares denote the diffusion coefficient at a particular shear rate, and the solid line depicts the linear fit. The dotted lines depict one standard deviation.

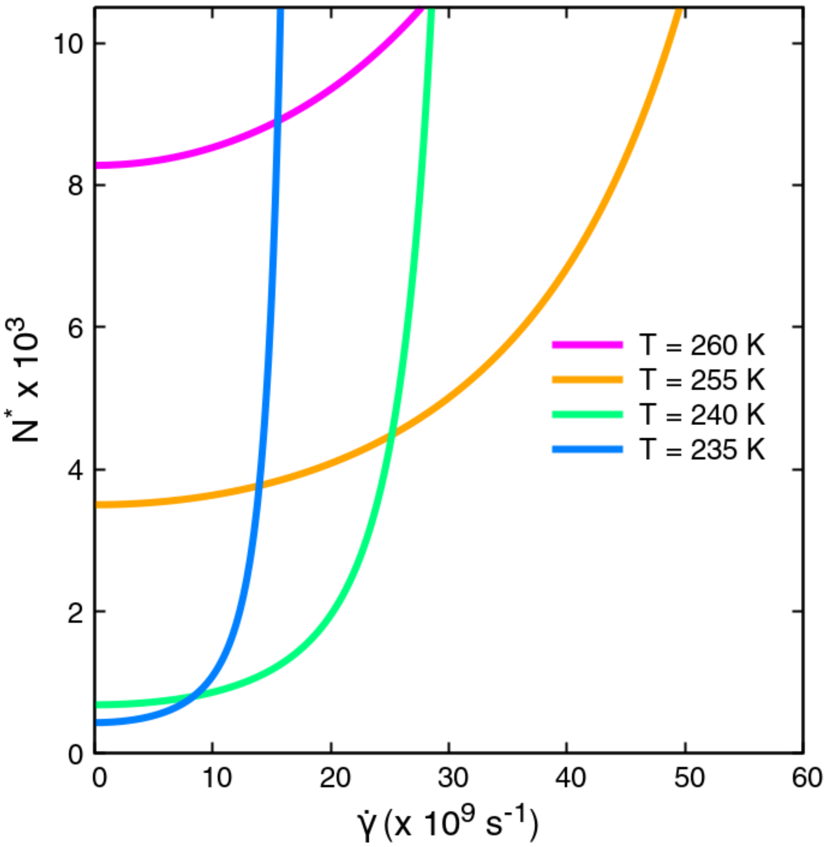


Figure S4: Variation of the cluster size $N^*$ with the shear rate $\dot{\gamma}$ for different temperatures. The increase is echoed by the increase in the height of the free energy barrier $F(N^*)$.

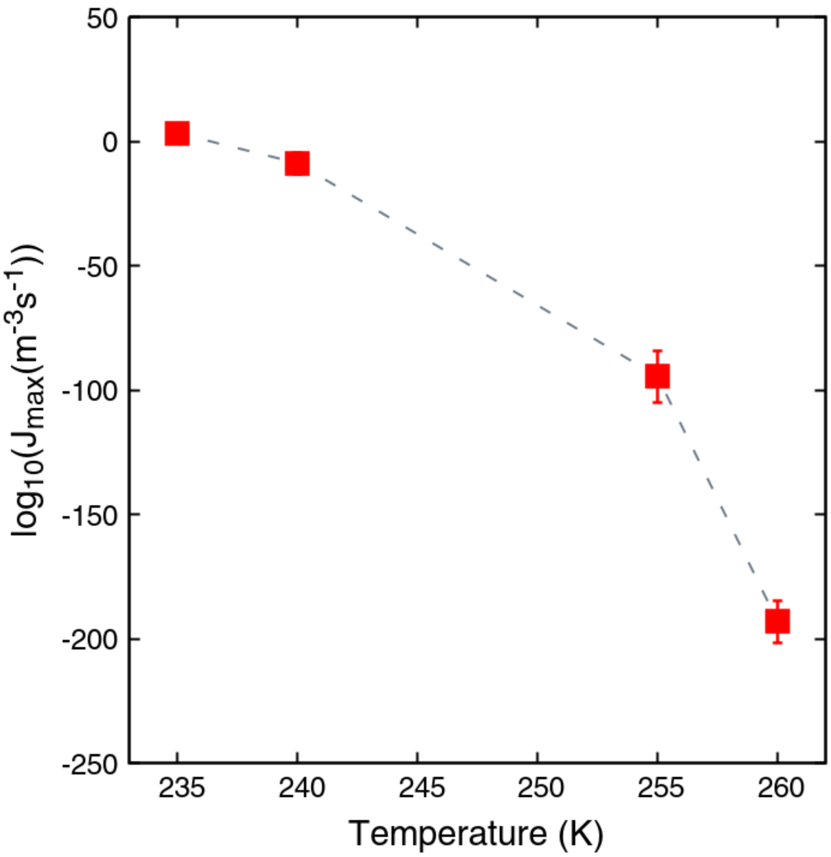


Figure S5: Logarithm of the maximum nucleation rate $J_{max}$, for each temperature studied in this work. The data points are represented by the red filled square symbols. The nucleation rate is higher for larger supercooling.

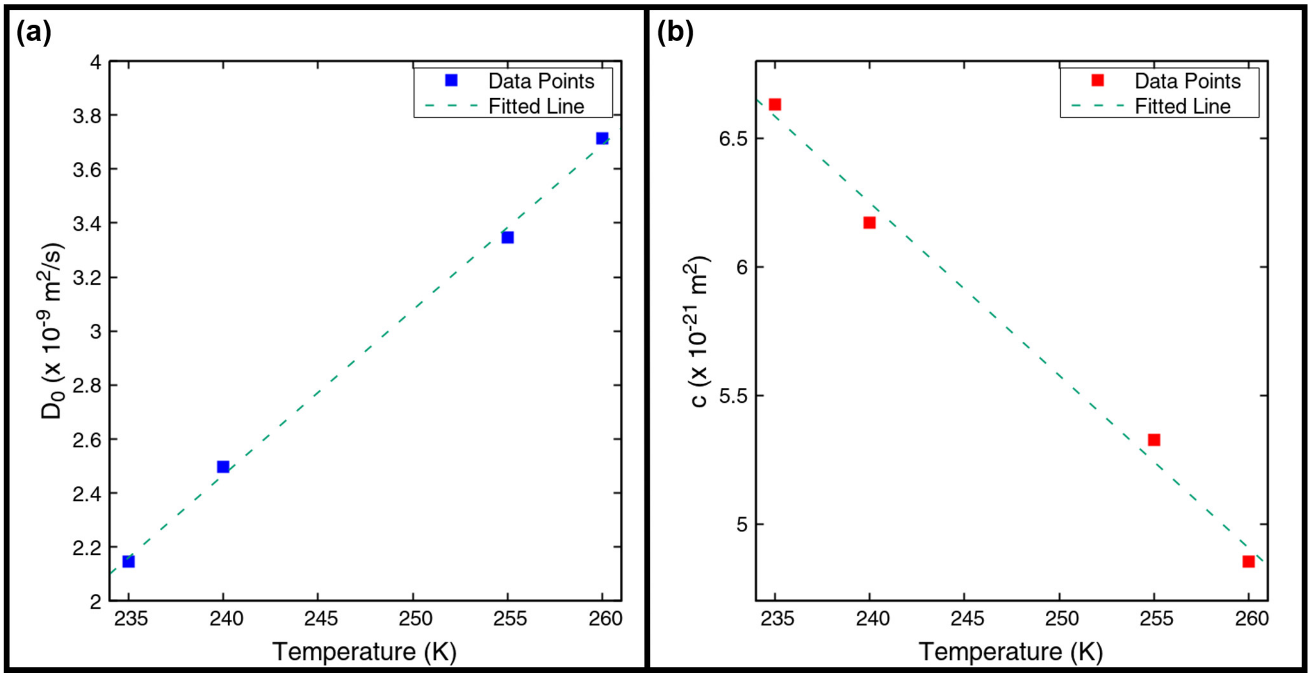


Figure S6: (a) Linear fit of the diffusion coefficient in the absence of shear $D_0$, plotted against the temperatures. The $D_0$ values obtained from simulations, and the fitted line are denoted by filled blue squares and a dotted slate-grey line, respectively. (b) Estimated linear relationship between the fitting parameter $c$ and the temperature. Filled red squares depict the the values of $c$ at 235, 240, 255 and 260 $K$. The line fitted to the data is shown as a dotted light-blue line. The calculated $D_0$ and $c$ values are listed in Table 4.1.

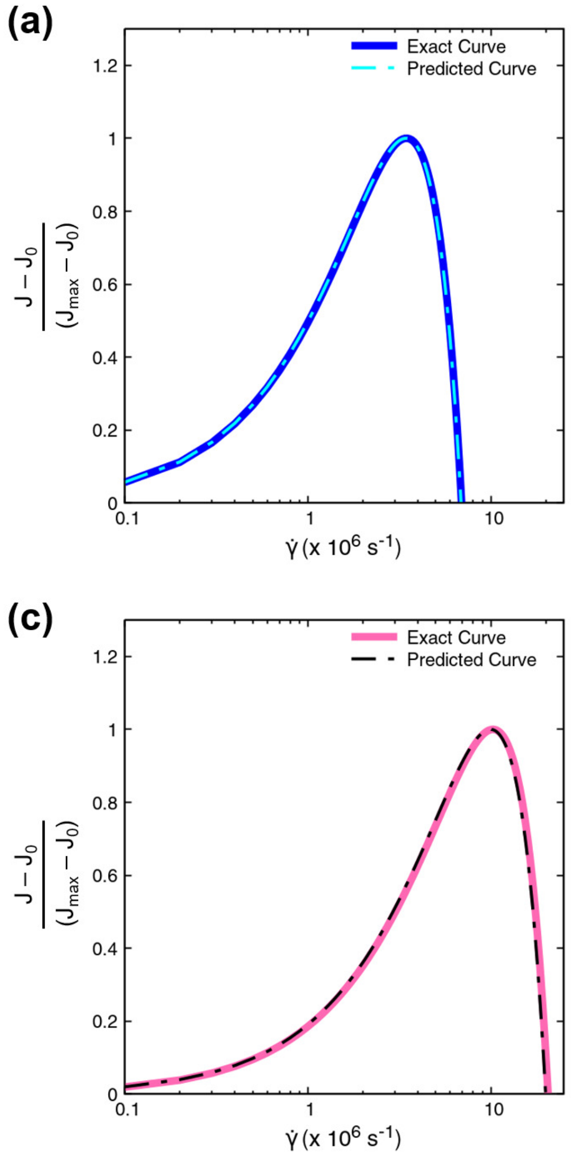


Figure S7: Predicted and exact normalized relative nucleation curves $\frac{J-J_0}{J_{max}-J_0}$, plotted against the shear rate $\dot{\gamma}$, for a) 235 K, (b) 240 K, (c) 255 K and (d) 260 K. Here, $J_0$ and $J_{max}$ are the nucleation rate in the absence of shear and the maximum nucleation rate at each temperature, respectively. In each plot, the solid lines denote nucleation rate curves calculated using seeded simulations, and the dotted lines depict the predicted nucleation curves estimated using approximations.

# References


(S1) Bai, X.-M.; Li, M. Test of classical nucleation theory via molecular-dynamics simulation. *The Journal of Chemical Physics* **2005**, *122*, 224510.

(S2) Bai, X.-M.; Li, M. Calculation of solid-liquid interfacial free energy: A classical nucleation theory based approach. *The Journal of Chemical Physics* **2006**, *124*, 124707.

(S3) Molinero, V.; Moore, E. B. Water Modeled As an Intermediate Element between Carbon and Silicon†. *The Journal of Physical Chemistry B* **2009**, *113*, 4008–4016.

(S4) Espinosa, J. R.; Sanz, E.; Valeriani, C.; Vega, C. Homogeneous ice nucleation evaluated for several water models. *The Journal of Chemical Physics* **2014**, *141*, 18C529.

(S5) Espinosa, J. R.; Vega, C.; Valeriani, C.; Sanz, E. Seeding approach to crystal nucleation. *The Journal of Chemical Physics* **2016**, *144*, 034501.

(S6) Dehaoui, A.; Issenmann, B.; Caupin, F. Viscosity of deeply supercooled water and its coupling to molecular diffusion. *Proceedings of the National Academy of Sciences* **2015**, *112*, 12020–12025.

(S7) Cao, P.; Wu, J.; Zhang, Z.; Fang, B.; Peng, L.; Li, T.; Vlugt, T. J. H.; Ning, F. Mechanical properties of bi- and poly-crystalline ice. *AIP Advances* **2018**, *8*, 125108.

(S8) Loerting, T.; Giovambattista, N. Amorphous ices: experiments and numerical simulations. *Journal of Physics: Condensed Matter* **2006**, *18*, R919–R977.

(S9) Moreira, P. A. F. P.; de Aguiar Veiga, R. G.; de Koning, M. Elastic constants of ice Ih as described by semi-empirical water models. *The Journal of Chemical Physics* **2019**, *150*, 044503.
